# Supplementary material for: Temperature-stabilized differential amplifer for low-noise DC measurements
Source: arXiv:1708.06311 ancillary file (2017-08-21)
Supplement: Supplementary file 1 [file 20170619a_supplemental_iterative_trimmer.pdf]

# Supplemental Material: Iterative Trimming

This is a description how to precisely adjust a resistor. For stability and noise performance we use an assembly of fixed value resistors instead of trimmers or potentiometers.
This technique is used in the amplifier presented in "Temperature-stabilized differential amplifier for low-noise DC measurements", Rev. Sci. Instrum.

A resistor can be precisely tuned by placing additional resistors in parallel. We present a technique using 4 parallel resistors, of which two are in series (A and B, Fig. 4). We use a potentiometer parallel to the existing resistor to get the target resistance, which will be placed next. We use a python script (Fig. 3) to successively determine the ideal values of A and B, then C, and later D. Depending on the initial error of resistor E, we reduce the error by two to three orders of magnitude by placing the resistors A and B, and one to two orders of magnitude each for C and D.

Remark: For higher accuracy, B should have a significantly lower resistance than A. This allows for a more accurate tuning using C and D).

Example: Adjust the voltage offset of the first amplification stage.

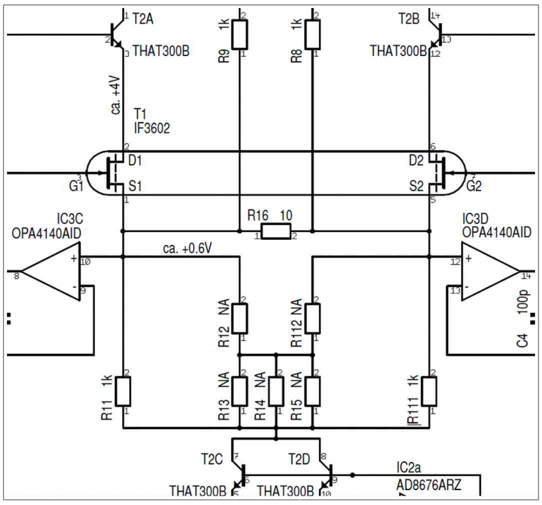


*Fig. 1: Schematic showing the resistors for offset adjustment of the first amplification stage.*

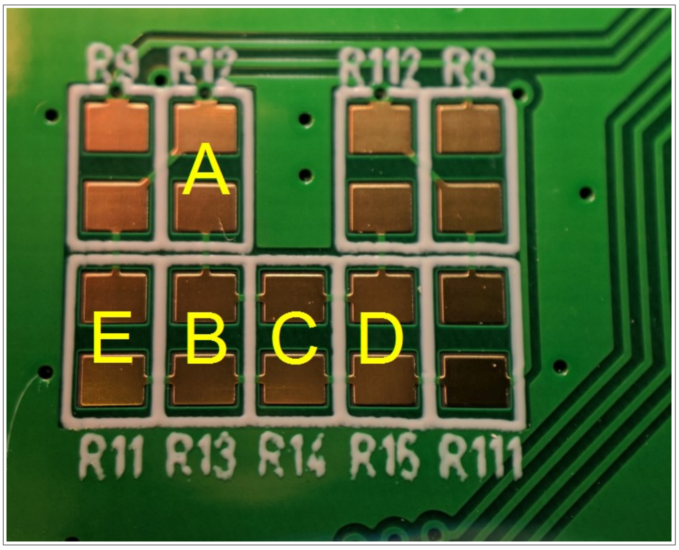


*Fig. 2: Circuit board.*

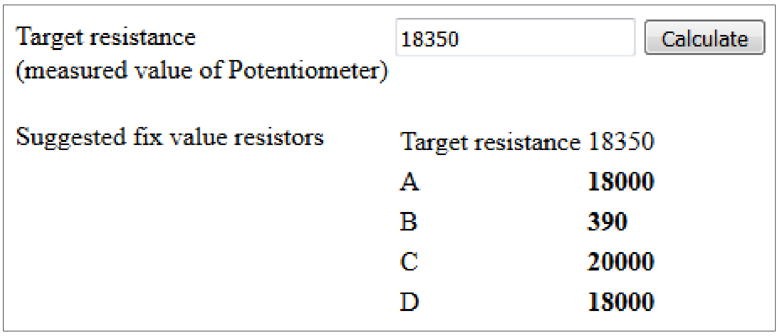


*Figure 3: Interface of python script.The script can be viewed and used on [www.positron.ch/iterativetrimmer](www.positron.ch/iterativetrimmer).*

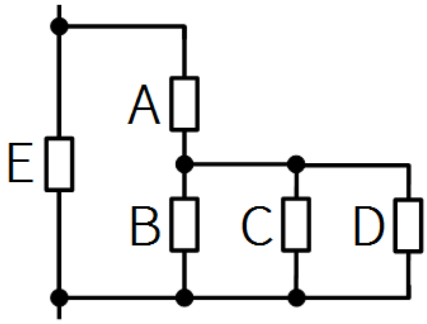


*Fig. 4: Schematic of general resistor assembly.*

R11 and R111 are already assembled. Let us further assume the resistance of the left branch (R11) has to be reduced to compensate the offset. The yellow letters in Fig. 2 show where we place the adjustment resistors A to D. R11 is resistor E in this case.

Example procedure:

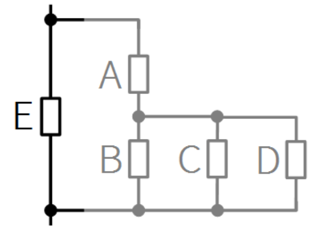


The resistance should be reduced. E is already assembled.

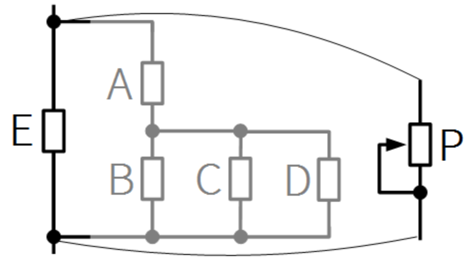


Trimmer P is connected temporary and adjusted until offset is zero.
Trimmer is removed and it's resistance P is measured.

Target resistance: 18315 = P
Result of python script:
**A: 18000**
**B: 360**
C: 20000
D: 18000

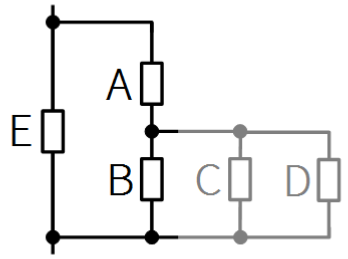


Assembling of resistors
**A: 18000**
**B: 360**

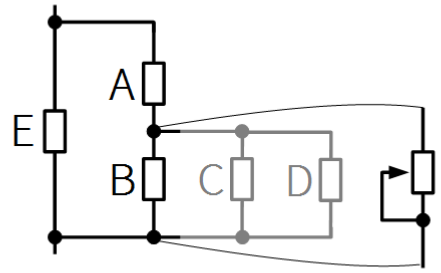


Trimmer P is adjusted until offset is zero.
Trimmer is removed and it's resistance P is measured.

Target resistance: 5700 = P
Result of python script:
A: 5600
B: 110
**C: 6200**
D: 5600

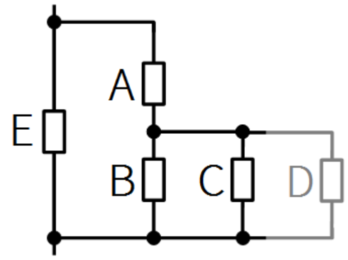


Assembling of resistor
**C: 6200**

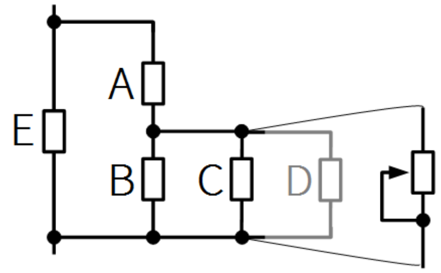


Trimmer P is adjusted until offset is zero.
Trimmer is removed and it's resistance P is measured.

Target resistance: 830000
Result of python script:
A: 820000
B: 11000
C: 910000
**D: 820000**

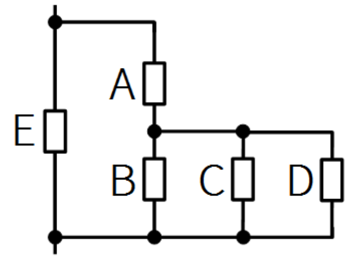


Assembling of resistor
**D: 820000**

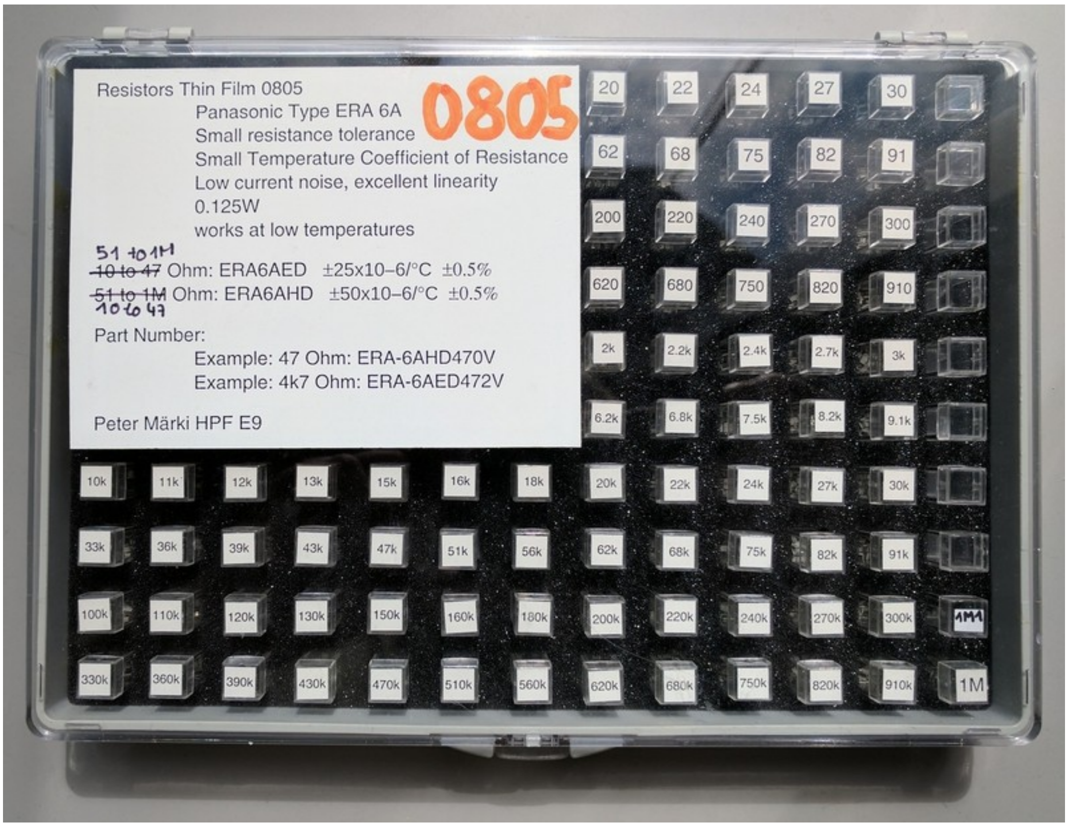


*Fig. 3: Resistor set, thinfilm, E24, values from 10 Ohm to 1 Mohm.*

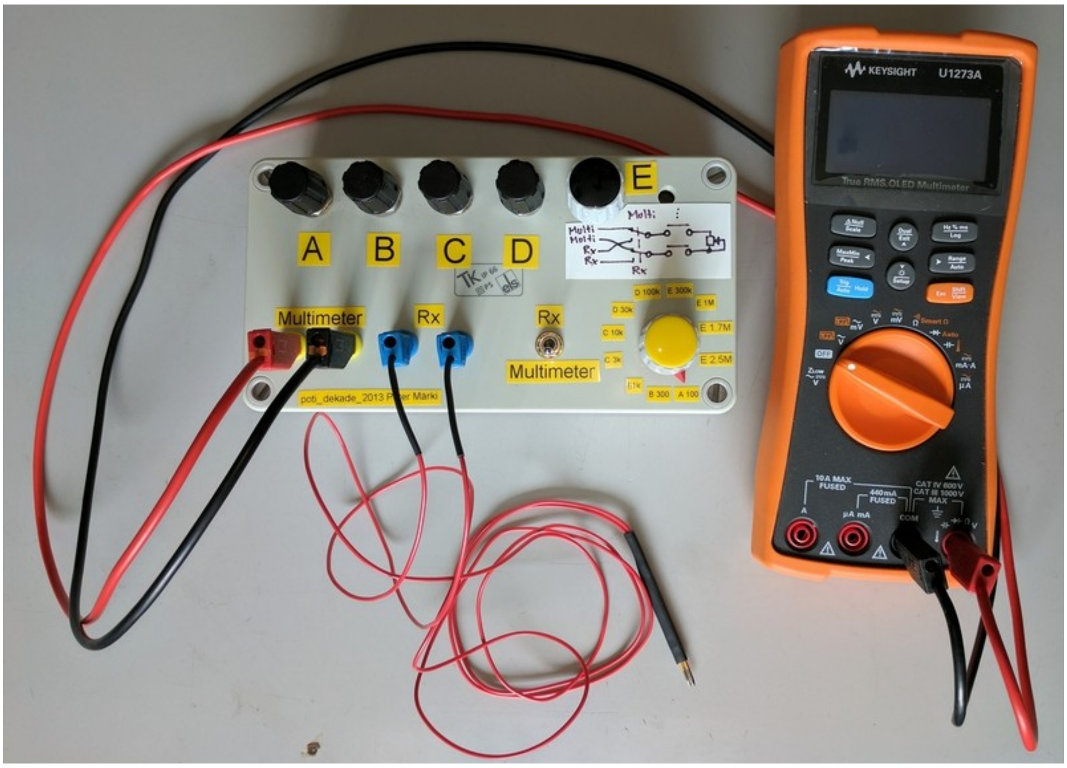


*Fig. 4: A device to speed up the trimming process. Switch to Rx, test-pins pressed on the circuit board, adjusting a trimmer (letters A to E on trimmers have nothing to do with resistors A to E). The range can be selected. Switch to Multimeter. Reading the resistance of the trimmer from the multimeter.*

Typically this concept works directly down to the ppm-range of the initial offset. Each iteration corrects errors from the previous iteration (potentiometer, resistance measurement, fix value resistor error).

If less accuracy is needed, the concept can be simplified by using only C and D for example.
