# Supplementary material for: Temperature-stabilized differential amplifer for low-noise DC measurements
Source: arXiv:1708.06311 ancillary file (2017-08-21)
Supplement: Supplementary file 2 [file 20170619a_supplemental_large_step_response.pdf]

# Supplemental Material: Large Step Response

This is a description of the amplifiers response to large signal steps at the input. Both symmetric and asymmetric signals typically have an influence on the FET temperature and cause a slowly varying offset voltage after large steps. The amplifier presented in "Temperature-stabilized differential amplifier for low-noise DC measurements", Rev. Sci. Instrum. keeps the power loss constant and therefore this type of response is small.

## 1 Response to common voltage step

A hard test is to step the common mode voltage and observe the reaction of the amplifier.

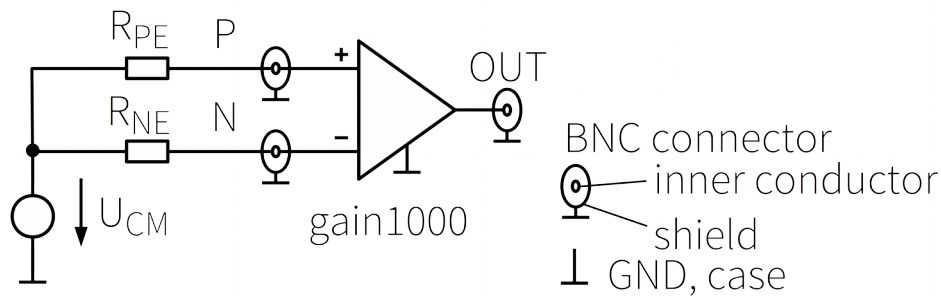

Figure 1: Test setup: Resistors  $R_{PE}$  and  $R_{NE}$  are connected to the amplifiers input. The common mode voltage  $U_{CM}$  is changed abruptly.

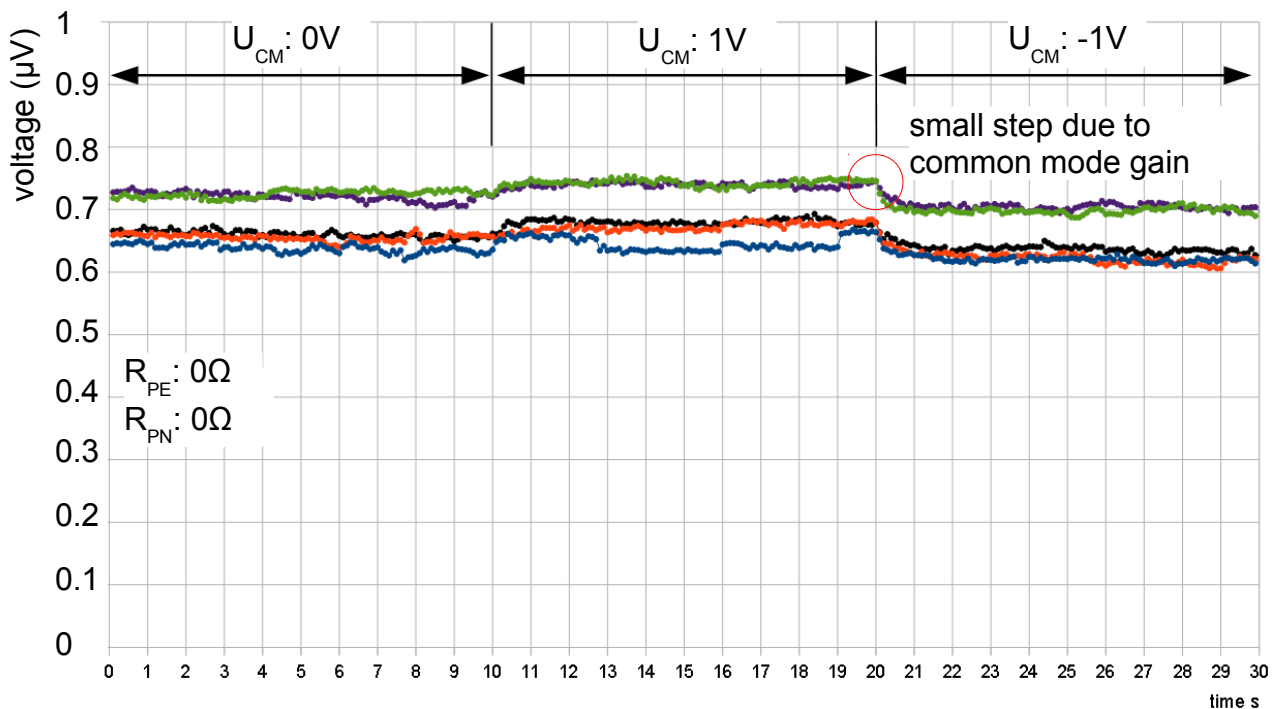

Figure 2: Test of common-mode step without resistors at the inputs: The output voltage of the amplifier is measured and the input error voltage is calculated. The measurement is repeated 5 times with a delay of 1h. Integration time: 0.1s.

With  $0\Omega$  input resistance, input voltage noise and common mode gain is visible. The change of the common mode voltage from 1V to -1V results in a step of about 50 nV. The CMMR (common-mode rejection ratio) is therefore  $2V / 50nV = 4 \cdot 10^7$  (150 dB).

Conclusion: the amplifier is not sensitive to common mode voltage steps.

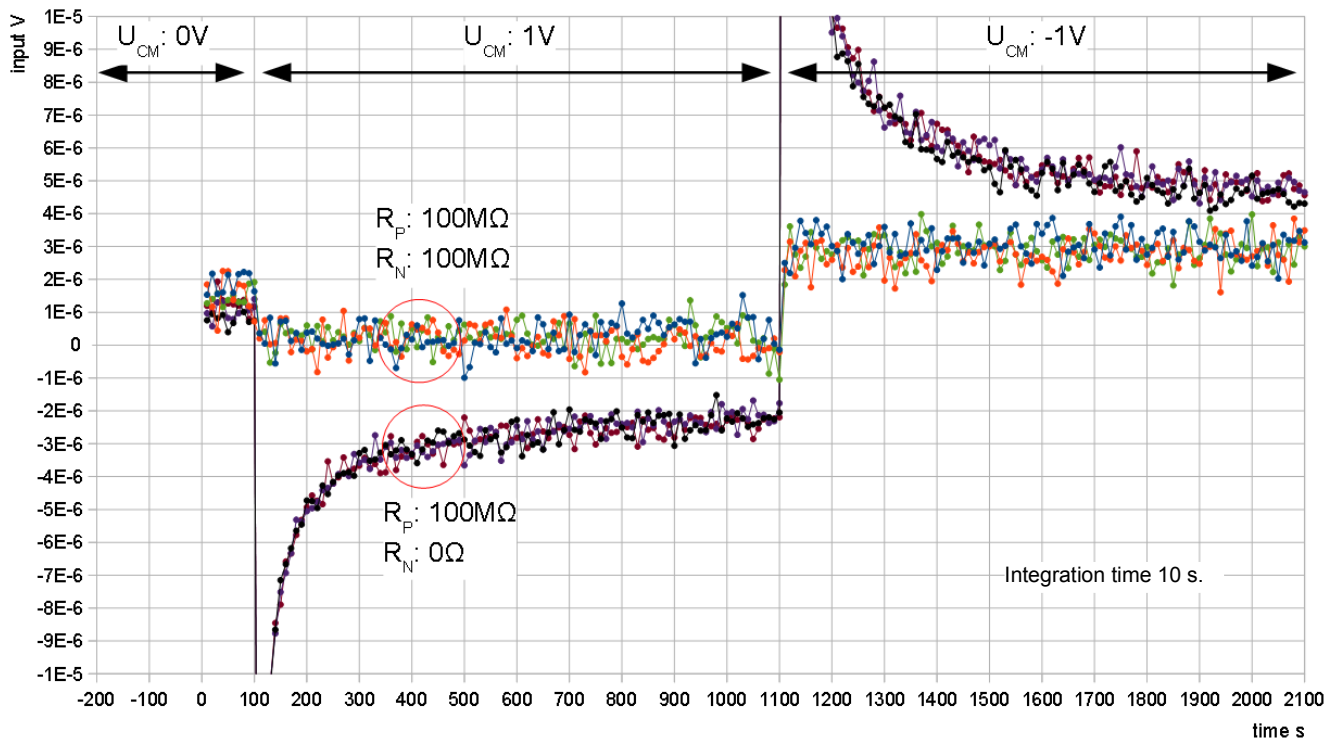

Figure 3: Test of common-mode step with 100MΩ resistors (symmetric and asymmetric) at the inputs: The output voltage of the amplifier is measured and the input error voltage is calculated. The measurement for every resistor combination is repeated 5 times with a delay of 1h.

With a 100 MΩ resistance connected to one or both inputs, the resistor noise (Johnson noise) and the amplifiers input current is the dominant error source. In the asymmetric case of 100 MΩ and 0Ω a slow equilibration is visible. The leakage currents are of the order of 50 fA. We assume that the varying leakage current stems from leakage in the insulation layer of the circuit board.

Conclusion: The common mode voltage has little influence on the leakage current. Compared to other amplifiers, this effect is significantly smaller.

## 2 Response to large signal step

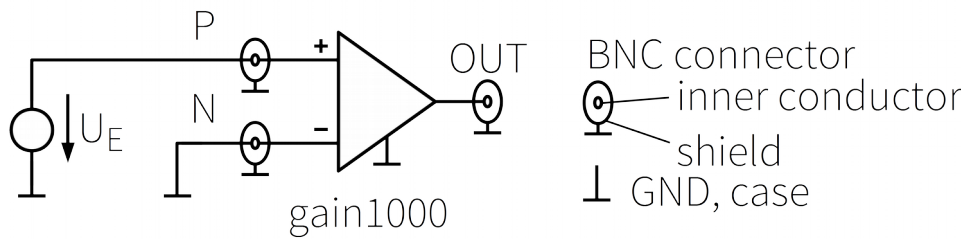

Figure 4: Test setup: Voltage  $U_E$  is changed abruptly.

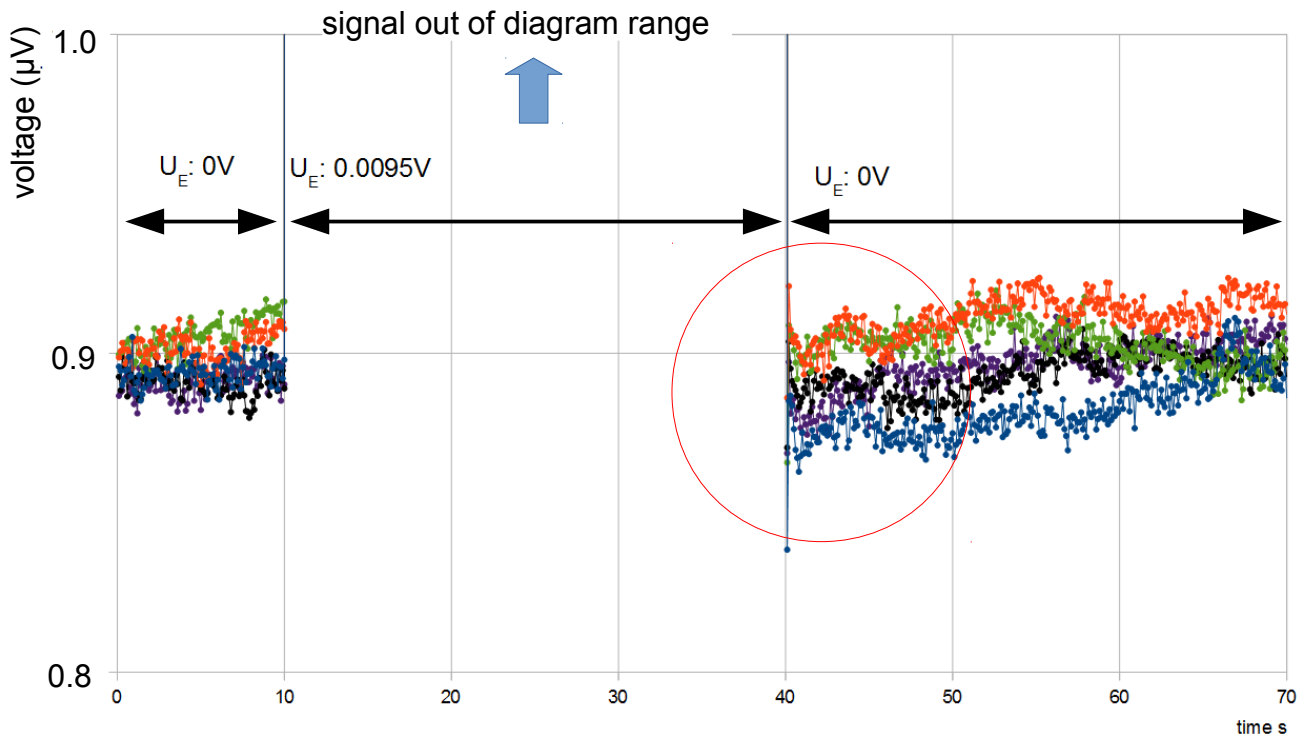

Figure 5: The input voltage is changed abruptly and the output voltage is measured. The input voltage is calculated by dividing the output voltage by the amplification factor. The measurement is repeated 5 times with a delay of 120s. Integration time is 0.1 s.

As shown in Fig. 5, after the input step from 9.5 mV to 0 mV the output voltage returns to zero without slow equilibration (highlighted by red circle).

Conclusion: The amplifier offset is unchanged even after large signal steps.
